# Supplementary material for: GASCN: Graph Attention Shape Completion Network
Source: arXiv:2201.07937 source file (2022-01-20)
Supplement: Supplementary file 1 [file appendix.tex]

\documentclass[10pt,twocolumn,letterpaper]{article}

\usepackage{3dv}
\usepackage{times}
\usepackage{epsfig}
\usepackage{graphicx}
\usepackage{amsmath}
\usepackage{amssymb}

% Include other packages here, before hyperref.
\usepackage[english]{babel}
\usepackage[utf8]{inputenc}

\usepackage{subcaption}
\usepackage[font = rm]{caption}
\usepackage{enumitem}
\usepackage[english]{babel}
\usepackage[utf8]{inputenc}
\usepackage{subcaption}
\usepackage[font = rm]{caption}

%\maketitle
% \thispagestyle{empty}
%\section{Appendix}
\setcounter{figure}{10}
\begin{figure*}
    \centering
    \small\textbf{Input\;\;\;\;\;\;\;\;\;\;\;\;\;\;\;\;\;FoldingNet\;\;\;\;\;\;\;\;\;\;\;\;\;\;\;\;\;TopNet\;\;\;\;\;\;\;\;\;\;\;\;\;\;\;\;\;GRNet\;\;\;\;\;\;\;\;\;\;\;\;\;\;\;\;\;\;PCN\;\;\;\;\;\;\;\;\;\;\;\;\;\;\;\;\;\;\;\;Ours\;\;\;\;\;\;\;\;\;\;\;\;\;\;\;\;\;Ground Truth}
    \includegraphics[width=1.0\textwidth]{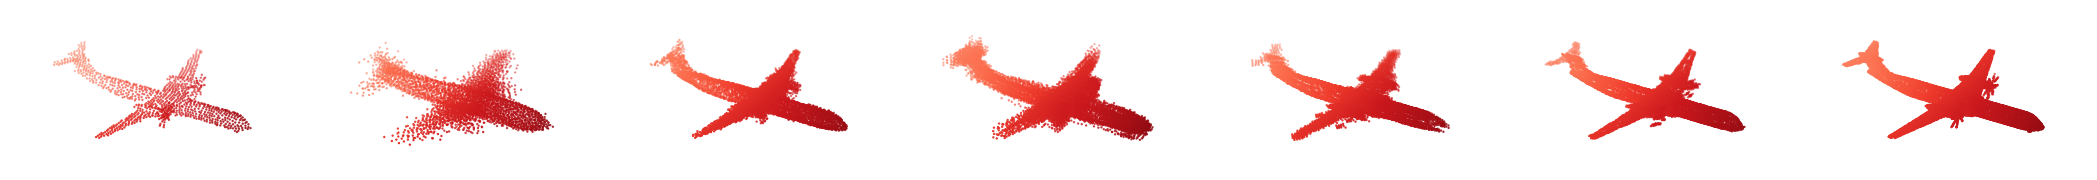}
    \includegraphics[width=1.0\textwidth]{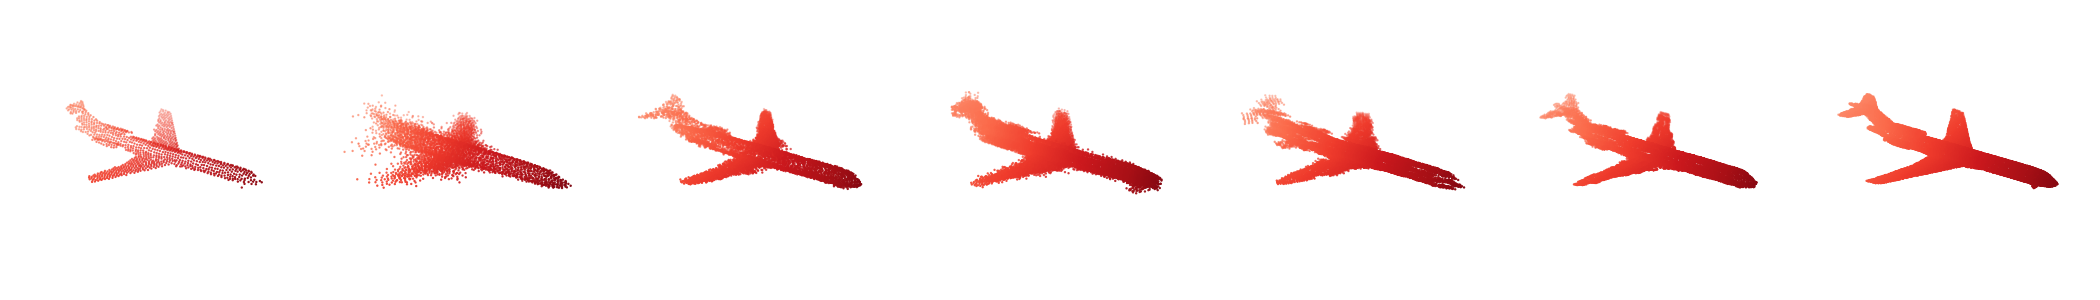}
    \includegraphics[width=1.0\textwidth]{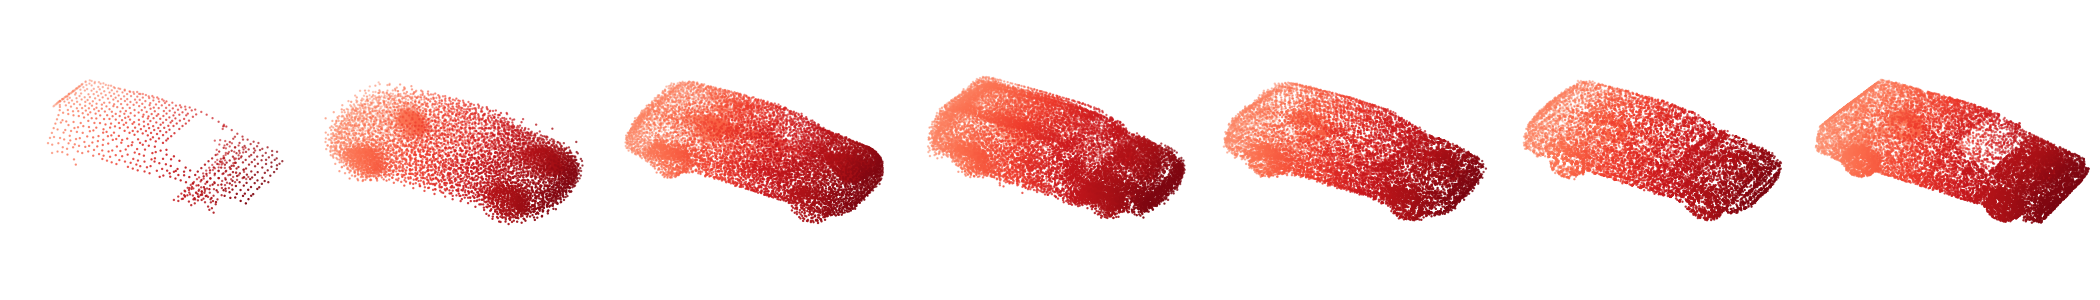}
    \includegraphics[width=1.0\textwidth]{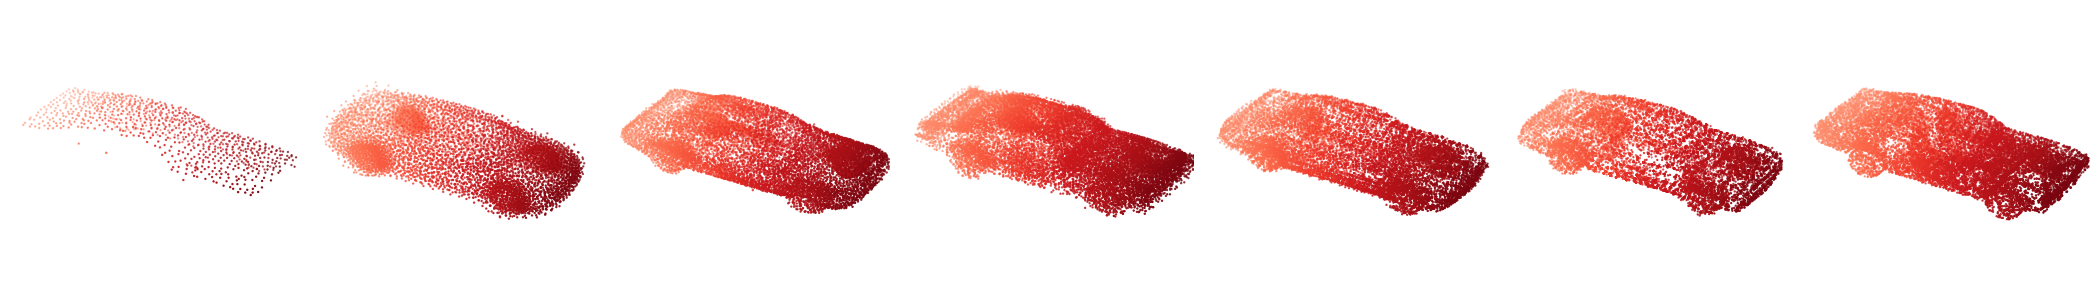}
    \includegraphics[width=1.0\textwidth]{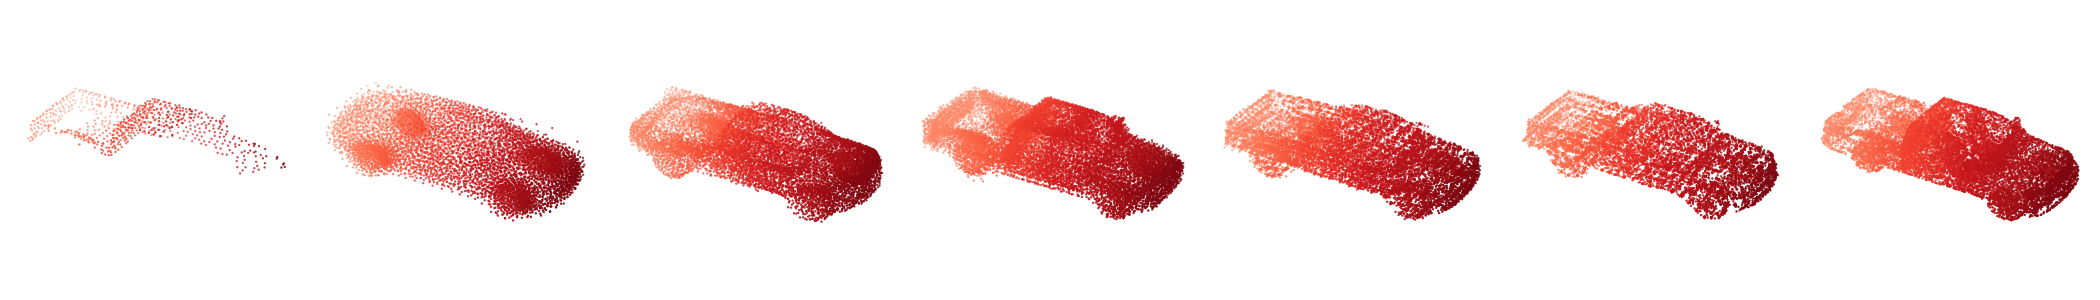}
    \includegraphics[width=1.0\textwidth]{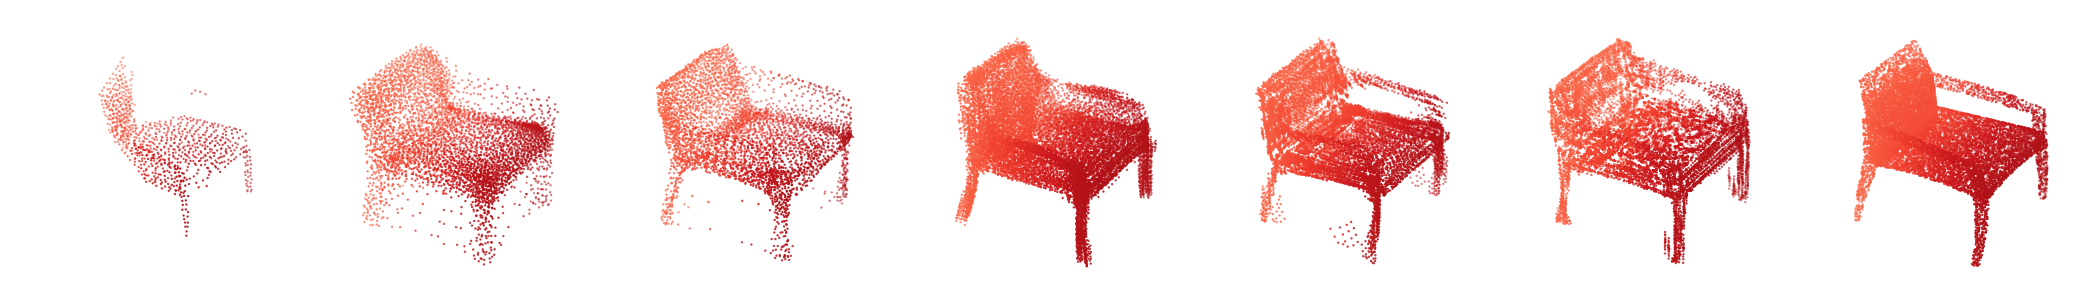}
    \includegraphics[width=1.0\textwidth]{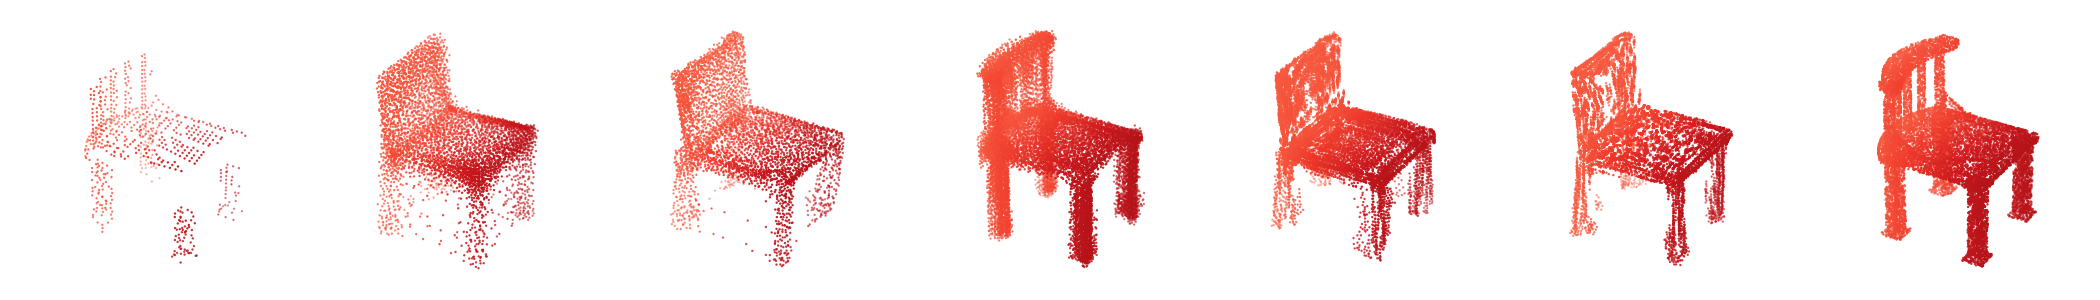}
    \includegraphics[width=1.0\textwidth]{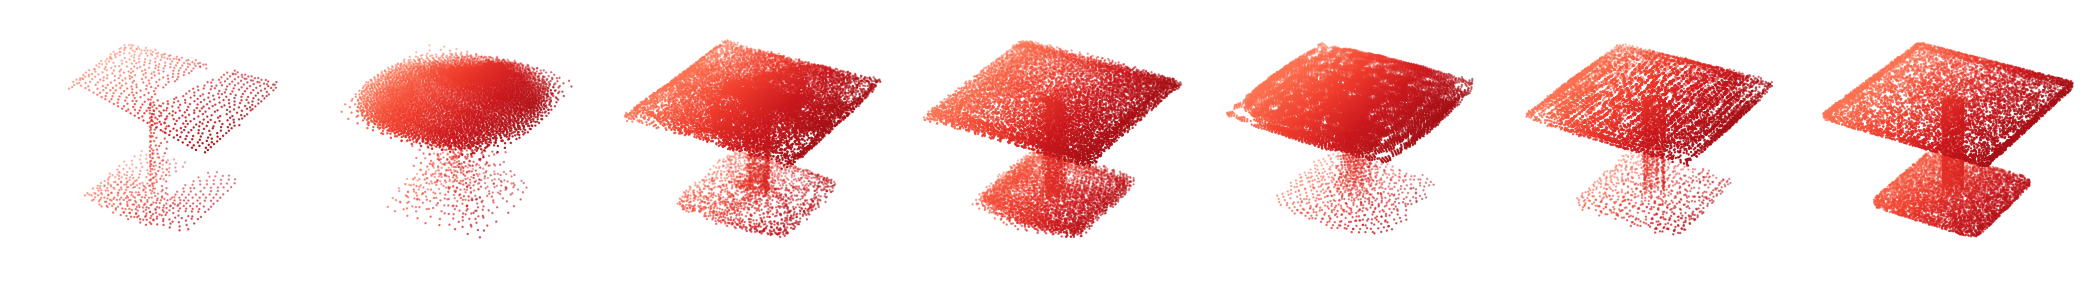}
    \includegraphics[width=1.0\textwidth]{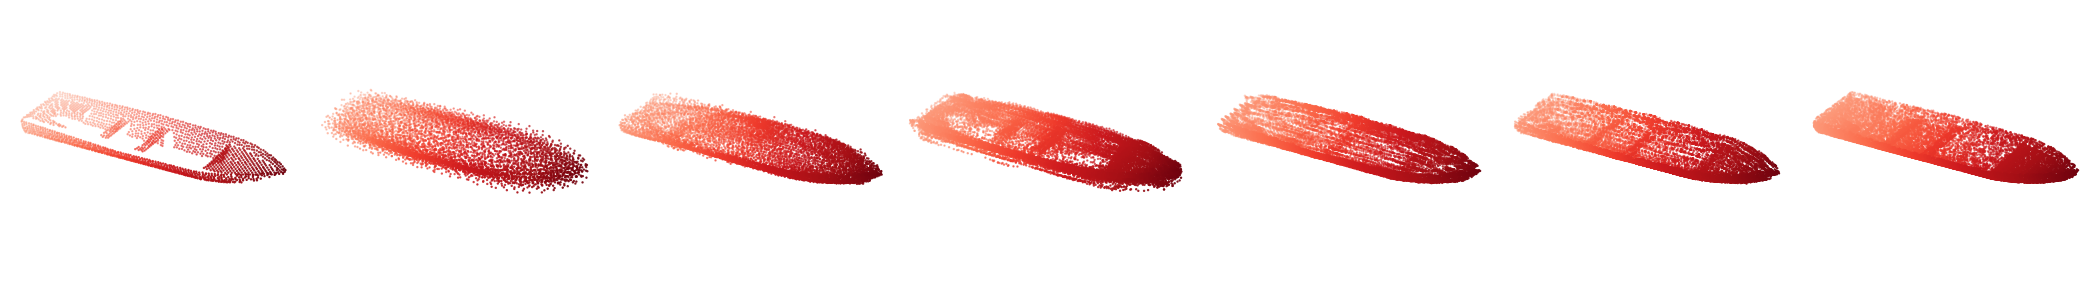}
    \caption{\textbf{More Qualitative Results Comparison.} A partial point cloud is given and our method generates better complete point clouds.}
\end{figure*}

\begin{figure*}[!htbp]
    \centering
    \includegraphics[scale=1.]{LaTex/more_compare_results/Copy of architecture.jpg}
    \caption{\textbf{Detailed Overview of Our Network Architecture.} The left part is our encoder and the right half part is our decoder. The size of the tensor is based on our experiment setting}
\end{figure*}
